# Supplementary material for: Deep Variational Reinforcement Learning for POMDPs
Source: arXiv:1806.02426 source file (2018-06-06)
Supplement: Supplementary file 1 [file 8_appendix.tex]

\section{Derivation of \gls{ELBO} loss}
\label{sec:ap:elbo}
Blub...

The loss $\mathcal{L}^{\text{ELBO}}_t(\theta,\phi)$ serves to maximise the average conditional \gls{ELBO} on
the $n_s$ observations received since the last update in each of the $n_e$ environments:
\begin{multline}
 \frac{1}{n_en_s} \sum_{\text{envs}}^{n_e} \ELBO_\text{SMC}(o_{t:t+n_s-1}|o_{<t}, a_{\le t+n_s-1}) =\\
  \frac{1}{n_en_s}\sum_{\text{envs}}^{n_e} \mathbb{E}_q\left[\left. \sum_{i = 0}^{n_s - 1} \log\left(\frac{1}{K} \sum_{k =
          1}^K w_{t + i}^k \right)\right| o_{<t}, a_{\le t+n_s-1}\right]  \label{eq:n-step-elbo}
\end{multline}

Blub...

Here we will show that equation \ref{eq:n-step-elbo} can be used for learning
models $p_\theta(z_{t+1}^k \given h_{t}^k \varphi^a_{\theta}(a_{t}))$ and $p_\theta(o_{t+1} \given z_{t+1}^k, \varphi_{a,\theta}(a_{t}))$
 as well as the approximate posterior $q_\theta(z_{t+1}^k|h_t^k, \varphi^a_{\theta}(a_t), \varphi^o_{\theta}(o_{t+1}))$.

 Our objective is
\begin{equation}
\label{eq:kl-objective}
\min_\theta D_{KL}\left[ P_{\mathcal{D}}(o_{1:T}, a_{0:T-1} \given \phi, \theta') \Vert P_\theta(o_{1:T}, a_{0:T-1}) \right]
\end{equation}

where $P_{\mathcal{D}}(o_{1:T},a_{0:T-1}\given \phi, \theta') = \int b_0(s_0) \prod_{t=1}^T
F(s_{t}|s_{t-1},a_{t-1}) U(o_t|s_t,a_{t-1}) \pi_\phi(a_t \given o_{\le t}, a_{<
  t}, \theta') ds_{0:T}$ is the distribution over observed trajectories under
policy $\pi$. Note that in our case $\pi$ is both directly parameterised by
$\phi$, but also depends on $\theta'$ through the latent state $\hat{b}_t(o_{\le
  t}, a_{<t}, \theta')$ that is used to aggregate the past history $(o_{\le t},
a_{< t})$ and on which it is conditioned in practise.

While one could use a fixed policy or parameters $\phi, \theta'$ for data
collection, we want our model to adapt to the learned policy. Consequently, we
will set $\theta'=\theta$ after each update to $\theta$. This also saves us from
computing both $\hat{b}_t(o_{\le t}, a_{<t}, \theta')$ (for the policy) and
$\hat{b}_t(o_{\le t}, a_{<t}, \theta)$ (for the optimisation).
\textcolor{gray}{As mentioned in the main text, we will accept a small in the gradients bias by 
assuming $\hat{b}_t(\theta)=\hat{b}_t(\theta + \Delta \theta)$ after each update step $\theta
\leftarrow \theta + \Delta \theta$.}

\textcolor{gray} The optimisation is only w.r.t to $\theta$, not $\theta'$: We
want to optimise the model given a policy but update the policy w.r.t the control
problem. (More explicity the interleaving?)

\subsection{Conditioning the \gls{ELBO} on actions}

Note that while we cannot evaluate $P_{\mathcal{D}}(o_{1:T},a_{0:T-1}\given \phi, \theta')$,
we can sample from it.

We will denote $P_{\mathcal{D}}=\Pdata$ and $Q(z_{0:T})=\Q$

<Signposts>
(Conditioning on action, deterministic internal computation, n-step loss,
particle filter, resampling = correct form). Also why strange writing of $\pi$

We can rewrite equation \ref{eq:kl-objective} as

\begin{equation}
\begin{split}
  & \max_\theta \int dP_{\mathcal{D}} \log \left[ \frac{P_\theta(o_{1:T}, a_{0:T-1})}{P_{\mathcal{D}}} \right] \\
  = & \max_\theta \int dP_{\mathcal{D}} \int dQ_\theta(z_{0:T}) \left\{ \log \left[ \frac{P_{\theta,\phi}(o_{1:T}, a_{0:T-1}, z_{0:T}) }{P_{\theta,\phi}(z_{0:T}|o_{1:T}, a_{0:T-1})}\frac{ Q_\theta(z_{0:T})} { Q_\theta(z_{0:T})} \right]  - \log P_{\mathcal{D}} \right\}\\
  = & \max_\theta \int dP_{\mathcal{D}} \int dQ_\theta(z_{0:T}) \left\{ \log \frac{P_{\theta,\phi}(o_{1:T}, a_{0:T-1}, z_{0:T})} {Q_\theta(z_{0:T})} + D_{\text{KL}}\left[ Q_\theta(z_{0:T})\Vert P_{\theta,\phi}(z_{0:T}|o_{1:T},a_{0:T-1})\right] - \log P_{\mathcal{D}} \right\} \\
  \ge & \max_\theta \int dP_{\mathcal{D}} \int dQ_\theta(z_{0:T})_{\theta,\phi} \left\{ \log \frac{P_{\theta,\phi}(o_{1:T}, a_{0:T-1}, z_{0:T})} {Q_\theta(z_{0:T})} - \log P_{\mathcal{D}} \right\}  
\end{split}
\end{equation}

We write
\begin{equation}
\log \hat{Z}_{\theta}(z_{0:T}, o_{1:T}| a_{0:T-1}) = \log \frac{P_\theta(z_{0}) \prod_{t=1}^T P_\theta(z_t|z_{t-1},a_{t-1}) P_\theta(o_t|z_t,a_{t-1})} {Q_\theta(z_{0:T})}
\end{equation}

and 

\begin{equation}
\pi_\phi(a_{0:T-1}\given o_{\le T}, \theta) = \pi_0(a_0) \prod_{t=1}^T \pi_\phi(a_t|o_{\le t}, a_{<t}, \theta)
\end{equation}

and can write for the integrand

\begin{equation}
\begin{split}
  & \int dP_{\mathcal{D}} \int dQ_\theta(z_{0:T})_{\theta,\phi} \left\{ \log \frac{P_{\theta,\phi}(o_{1:T}, a_{0:T-1}, z_{0:T})} {Q_\theta(z_{0:T})} -\log P_\mathcal{D} \right\} \\
 = & \int dP_{\mathcal{D}} \int dQ_\theta(z_{0:T})_{\theta,\phi} \left\{ \log \hat{Z}_\theta(z_{0:T}, o_{1:T}\given a_{0:T-1}) + \log \frac{\pi_\phi(a_{0:T-1}\given o_{\le T}, \theta)} {\pi_\phi(a_{0:T-1}\given o_{\le T}, \theta')} - \log \frac{P_\mathcal{D}}{\pi_\phi(a_{0:T-1}\given o_{\le T}, \theta')} \right\} \\
 % = & \int P_{\mathcal{D}} \int Q_\theta(z_{0:T})_{\theta,\phi} \left\{ \log \hat{Z}_{z_{0:T}}(z_{0:T}\given a_{0:T-1}) \right\} do_{1:T} da_{0:T-1} - H_{\theta,\phi}(A_{0:T-1}|O_{\le T}) + H_{\theta',\phi}(A_{0:T-1}|O_{\le T}) + H_{\theta'}(O_{\le T})\\
 = & \int dP_{\mathcal{D}} \int dQ_\theta(z_{0:T})_{\theta,\phi} \left\{ \log \hat{Z}_{\theta}(z_{0:T}, o_{1:T}\given a_{0:T-1}) \right\}  - D_{\text{KL}}\left[ \pi_\phi(a_{0:T-1}\given o_{\le T}, \theta') \Vert \pi_\phi(a_{0:T-1}\given o_{\le T}, \theta) \right] + H_{\theta'}(O_{\le T})\\
 = &  \int dP_{\mathcal{D}} \int dQ_\theta(z_{0:T})_{\theta,\phi} \left\{ \log \hat{Z}_{\theta}(z_{0:T}, o_{1:T}\given a_{0:T-1}) \right\} + H_{\theta'}(O_{\le T})
  % \log \frac{\pi(a_{0:T-1}\given o_{\le T}, \theta)} {\pi(a_{0:T-1}\given o_{\le T}, \theta')} - \log \frac{P_\mathcal{D}}{\pi(a_{0:T-1}\given o_{\le T}, \theta')}  do_{1:T} da_{0:T-1} \\
\end{split}
\end{equation}

where the last equality is due to $\theta=\theta'$. In other words, because we
have access to the policy, we can explain the entropy associated with the actions
and do not need to include them into our learned model. Furthermore, since the
KL-divergence is already 0, i.e. optimal, its gradient w.r.t $\theta$ is 0.

The observation entropy $H_{\theta'}(O_{\le T})$ is independent of $\theta$, so
we can ignore it when optimising the model. Consequently, our new objective is

\begin{equation}
\label{eq:ap:objective}
\max_\theta  \int d\Pdata \int d\Q \left\{ \log \hat{Z}_{z_{0:T}}(z_{0:T}, o_{1:T}\given a_{0:T-1}) \right\} 
\end{equation}

\subsection{Extending the generative model by deterministic computations}

So far we have assumed the action-conditioned generative model 

\begin{equation}
P_\theta(z_{0}) \prod_{t=1}^T P_\theta(z_t|z_{t-1},a_{t-1}) P_\theta(o_t|z_t,a_{t-1})
\end{equation}

However, we can easily use an extended model 

\begin{equation}
P_\theta(h_{0}) \prod_{t=1}^T P_\theta(z_t|h_{t-1},a_{t-1}) P_\theta(h_t| h_{t-1}, z_t, a_{t-1}) P_\theta(o_t|h_t,a_{t-1})
\end{equation}

Setting 

\begin{equation}
P_\theta(h_t| h_{t-1}, z_t, a_{t-1}) = \delta_{\psi_\theta^{\text{RNN}}(h_{t-1}, z_t, a_{t-1})}(h_t)
\end{equation}

with $\delta$ denoting the Dirac delta distribution allows us to include
deterministic computations in the model. This requires us to share the
parameters $\theta^{\text{RNN}}$ between the model and the posterior $Q(z_{1:T},
h_{0:T})$ which now takes the form \citep{chung2015recurrent}

\begin{equation}
\label{eq:vrnn-update}
Q(z_{1:T}, h_{0:T}| o_{1:T}, a_{0:T-1}) = q_\theta(h_0) \prod_{t=1}^T q_\theta(z_t | h_{t-1}, o_t, a_{t-1}) \delta_{\psi_\theta^{\text{RNN}}(h_{t-1}, z_t, a_{t-1})}(h_t)
\end{equation}

\subsection{Using the \gls{AESMC} objective}

The typical approach of estimating the integral over $dQ(z_{0:T})$ in equation
\ref{eq:ap:objective} by simple Monte Carlo sampling falls short for our use
case for three reasons:

First, the variance of the estimator grows exponentially (? \citep{doucet2009tutorial}) in the
length of the sequence $T$ which can be extremely large in \gls{RL}. Second, if
we want to condition our policy on the estimated latent state, we need to
capture the uncertainty of the posterior distribution. This is only possible
with a weighted set of particles when the \gls{ESS} (\toref) is not too low, i.e. when the
variance of the weights is not too high. In other words, we want most particles
to carry significant weight.

Lastly, this will be explained in detail in the next section, we want a loss
function that decomposes as a sum over time.

For those reasons, we will use \gls{AESMC}
\citep{le2018autoencoding,maddison2017filtering} to estimate $\int d\Q \left\{ \log
  \hat{Z}_{z_{0:T}}(z_{0:T}, o_{1:T}\given a_{0:T-1}) \right\}$. 

Comparing the generative model $p_\theta$, as well as $Q_{\SMC}$ and
$\hat{Z}_{\SMC}$ in \citet{le2018autoencoding} with our model $P_\theta$ leads
to the sampling procedure for $Q(z_{1:T}, h_{0:T})$ described in section
\ref{sec:recursive-update} which we repeat here:

\begin{align}
u_t^k & \sim \mathrm{Discrete}\left(\frac{w_{t}^k}{\sum_{j=1}^K w_t^j}\right)\\
z_{t+1}^k & \sim q_\theta(z_t^k|h_t^{u_t^k}, \varphi_{a,\theta}(a_t), \varphi_{o,\theta}(o_{t+1}))\\
h_{t+1}^k & = \psi_\theta^{RNN}(h_t^{u_t^k}, \varphi_\theta^z(z_{t+1}^k), \varphi_{a,\theta}(a_t), \varphi_{o,\theta}(o_{t+1})) \\
% w_{t+1}^k & = \frac{
% 	p_\theta(z_{t+1}^k \given h_{t}^{u_t^k}, \varphi^a_{\theta}(a_{t})) 
% 	p_\theta(o_{t+1} \given z_{t+1}^k, \varphi^a_{\theta}(a_{t}))}
% 	{q_\theta(z_{t+1}^k|h_t^{u_t^k}, \varphi^a_{\theta}(a_t), \varphi^o_{\theta}(o_{t+1}))} \label{eq:dvrl-w}
\end{align}

The sampling of $z_{t+1}$ and $h_{t+1}$ follows the same dependencies as in
equation \ref{eq:vrnn-update}, however, with an additional resampling step that
draws ancestor indices $u_t$. 

We can then compute the weights according to 
\begin{equation}
w_{t+1}^k = \frac{
	p_\theta(z_{t+1}^k \given h_{t}^{u_t^k}, \varphi^a_{\theta}(a_{t})) 
	p_\theta(o_{t+1} \given z_{t+1}^k, \varphi^a_{\theta}(a_{t}))}
	{q_\theta(z_{t+1}^k|h_t^{u_t^k}, \varphi^a_{\theta}(a_t), \varphi^o_{\theta}(o_{t+1}))}
\end{equation}

and compute the action-conditioned \gls{ELBO}

\begin{equation}
\begin{split}
  \ELBO_{\text{SMC}}(\theta, o_{\leq T} | a_{0:T-1}) & = \int d\Q \left\{ \log \hat{Z}_{z_{0:T}}(z_{0:T}, o_{1:T}\given a_{0:T-1}) \right\} \\
  & =  \E\left[\sum_{t = 1}^T\log \left(  \frac{1}{K} \sum_{k = 1}^K w_t^k \right)\right]
\end{split}
\end{equation}

For details we refer to \citet{le2018autoencoding}. 

Using the resampling step is key, not only to reduce the variance drastically,
but also to decompose the \gls{ELBO} into a sum over time. Compare the loss
function without resampling, purely based on \gls{IS} \citep{doucet2009tutorial,burda2016importance}

\begin{equation}
  \ELBO_{\text{IWAE}}(\theta, o_{\leq T} | a_{0:T-1}) = \E\left[ \log \left( \frac{1}{K} \sum_{k = 1}^K \prod_{t = 1}^T w_t^k \right)\right]
\end{equation}

The decomposition over time of $\ELBO_{\SMC}$ will be used in the next section.

\subsection{Stochastic Gradient Estimation}

In \gls{RL} the goal is to optimise the expected future return

\begin{equation}
  J = \mathbb{E}_{p(\tau)}\left[\sum_{t=1}^T \gamma^{t-1} r_t \right]
\end{equation}

over trajectories $\tau$. This can also be written as 

\begin{align}
  J & = \int d\rho^\pi(s) \int d\pi_\phi(a|s) r(s,a)\\
  \nabla_\phi J & = \mathbb{E}_{s\sim \rho^\pi, a\sim\pi_\phi}\left[ \nabla_\phi \log \pi_\phi(a|s) A(s,a) \right] \label{eq:ap:grad-J}
\end{align}

where $\rho^\pi(s)=(1-\gamma) \sum_{t=0}^t \gamma^t p^\pi(s_t)$ is the discounted state distribution
induced by policy $\pi$.

SGD

The $n$-step A2C gradient is computed by an approximation to equation
\ref{eq:ap:grad-J} by drawing $s$ from $n_e$ parallel environments for  

Bias in two ways

N-step learning?? But is the discounting done properly??

The integral $\int Q_\theta(z_{0:T}) \hat{Z}_{\theta,\phi}(z_{0:T})$ is an unbiased
estimator of the marginal likelihood of trajectories drawn from $P_\mathcal{D}$.
Consequently, due to Jensen's Inequality, $\int Q_\theta(z_{0:T}) \log
\hat{Z}_{\theta,\phi}(z_{0:T})$ is a lower bound for it.
When the bound is tight, $D_{\text{KL}}\left[ Q_\theta(z_{0:T})\Vert
  P_{\theta,\phi}(z_{0:T}|o_{1:T},a_{0:T-1})\right]=0$ and equality holds in the
last line.

This justifies to, instead of approximating it by simple Monte Carlo,
estimating it using a lower variance estimator $\int Q_\theta^{\SMC}(z_{0:T}) \log
\hat{Z}^{\SMC}_{\theta,\phi}(z_{0:T})$ \citep{le2018autoencoding,maddison2017filtering} which is particularly useful for
sequential data \citep{doucet2009tutorial}.
